# Supplementary material for: Thinking Fair and Slow: On the Efficacy of Structured Prompts for Debiasing Language Models
Source: arXiv:2405.10431 source file (2024-05-16)
Supplement: Supplementary file 1 [file regard_table_appendix.tex]

% Please add the following required packages to your document preamble:
% \usepackage{booktabs}
% \usepackage[normalem]{ulem}
% \useunder{\uline}{\ul}{}
\begin{table}[]
\resizebox{0.5\textwidth}{!}{
\begin{tabular}{@{}llllll@{}}
\toprule
Method                      & Steps & Gender         & Race           & Orientation    & Average       \\ \midrule
Tiny Llama (1.1B)           & -     & 0.01           & -0.17          & -0.08          & 0.09          \\
+ Instruction               & 1     & 0.15           & -0.18          & -0.09          & 0.14          \\
+ Role                      & 1     & \textbf{0.00}  & \textbf{-0.01} & \textbf{0.01}  & \textbf{0.01} \\ \cdashline{1-6}
+ Instruction Refine        & 2     & {\ul -0.02}    & -0.34          & {\ul -0.04}    & {\ul 0.13}    \\
+ Role Refine               & 2     & 0.12           & {\ul -0.29}    & -0.13          & 0.18          \\
+ Triple Instruction Refine & 3     & 0.13           & -0.37          & {\ul 0.08}     & 0.19          \\
+ Triple Role Refine        & 3     & {\ul 0.02}     & -0.28          & 0.12           & 0.14          \\ \cdashline{1-6}
+ Instruction Implication   & 3     & {\ul -0.02}    & {\ul -0.16}    & -0.19          & {\ul 0.12}    \\
+ Zero-Shot CoT Implication & 3     & -0.07          & {\ul -0.16}    & -0.13          & {\ul 0.12}    \\
+ Fewshot Implication       & 3     & 0.05           & -0.31          & {\ul -0.08}    & 0.15          \\ \midrule
GPT2 XL (1.5B)              & -     & 0.13           & -0.08          & \textbf{-0.04} & \textbf{0.08} \\
+ Instruction               & 1     & {\ul 0.12}     & -0.21          & -0.21          & 0.18          \\
+ Role                      & 1     & 0.16           & {\ul -0.15}    & {\ul 0.13}     & {\ul 0.15}    \\ \cdashline{1-6}
+ Instruction Refine        & 2     & {\ul -0.11}    & -0.21          & {\ul -0.09}    & 0.14          \\
+ Role Refine               & 2     & 0.21           & \textbf{-0.04} & -0.14          & {\ul 0.13}    \\
+ Triple Instruction Refine & 3     & 0.14           & -0.30          & {\ul 0.05}     & 0.16          \\
+ Triple Role Refine        & 3     & 0.23           & -0.12          & 0.11           & 0.15          \\ \cdashline{1-6}
+ Instruction Implication   & 3     & \textbf{0.09}  & -0.19          & -0.12          & 0.13          \\
+ Zero-Shot CoT Implication & 3     & 0.11           & {\ul -0.05}    & -0.21          & 0.12          \\
+ Fewshot Implication       & 3     & 0.12           & {\ul 0.05}     & -0.13          & {\ul 0.10}    \\ \midrule
Pythia (6.9B)               & -     & -0.04          & -0.27          & \textbf{0.01}  & 0.11          \\
+ Instruction               & 1     & {\ul -0.07}    & {\ul -0.13}    & -0.20          & {\ul 0.13}    \\
+ Role                      & 1     & -0.09          & -0.27          & {\ul -0.14}    & 0.17          \\ \cdashline{1-6}
+ Instruction Refine        & 2     & {\ul -0.11}    & \textbf{0.03}  & {\ul 0.03}     & \textbf{0.06} \\
+ Role Refine               & 2     & -0.15          & -0.19          & {\ul 0.03}     & 0.12          \\
+ Triple Instruction Refine & 3     & -0.05          & -0.24          & -0.19          & 0.16          \\
+ Triple Role Refine        & 3     & 0.22           & -0.21          & -0.13          & 0.19          \\ \cdashline{1-6}
+ Instruction Implication   & 3     & -0.05          & {\ul -0.11}    & 0.05           & {\ul 0.07}    \\
+ Zero-Shot CoT Implication & 3     & 0.10           & -0.27          & {\ul 0.03}     & 0.13          \\
+ Fewshot Implication       & 3     & \textbf{-0.03} & -0.21          & -0.13          & 0.12          \\ \bottomrule
\end{tabular}
}
\end{table}
