# Supplementary material for: Thinking Fair and Slow: On the Efficacy of Structured Prompts for Debiasing Language Models
Source: arXiv:2405.10431 source file (2024-05-16)
Supplement: Supplementary file 2 [file ss_table_appendix.tex]

% Please add the following required packages to your document preamble:
% \usepackage{booktabs}
% \usepackage[normalem]{ulem}
% \useunder{\uline}{\ul}{}
\begin{table}[]
\resizebox{0.5\textwidth}{!}{
\begin{tabular}{lllll}
\hline
Method                      & Steps & SS             & LM             & ICAT           \\ \hline
Tiny Llama (1.1B)           & -     & 61.60          & 87.48          & 67.19          \\
+ Instruction               & 1     & {\ul 61.91}    & {\ul 91.14}    & {\ul 69.42}    \\
+ Role                      & 1     & 63.70          & 91.09          & 66.14          \\ \cdashline{1-5}
+ Instruction Refine        & 2     & {\ul 58.62}    & 92.19          & {\ul 76.29}    \\
+ Role Refine               & 2     & 58.80          & \textbf{92.29} & 76.05          \\ \cdashline{1-5}
+ Triple Instruction Refine & 3     & 58.76          & 92.11          & 75.97          \\
+ Triple Role Refine        & 3     & 58.83          & \textbf{92.29} & 75.99          \\ \cdashline{1-5}
+ Instruction Implication   & 3     & \textbf{56.68} & 92.08          & \textbf{79.77} \\
+ Zero-Shot CoT Implication & 3     & 56.66          & 91.90          & 79.66          \\
+ Fewshot Implication       & 3     & 57.19          & 92.24          & 78.97          \\ \hline
GPT2 XL (1.5B)              & -     & 64.11          & 93.76          & 67.30          \\
+ Instruction               & 1     & 63.06          & 94.36          & 69.72          \\
+ Role                      & 1     & {\ul 61.60}    & \textbf{94.72} & {\ul 72.75}    \\ \cdashline{1-5}
+ Instruction Refine        & 2     & {\ul 59.84}    & 92.75          & 74.49          \\
+ Role Refine               & 2     & 60.16          & {\ul 93.66}    & \textbf{74.62} \\ \cdashline{1-5}
+ Triple Instruction Refine & 3     & 59.98          & 92.83          & {\ul 74.30}    \\
+ Triple Role Refine        & 3     & 60.34          & {\ul 93.61}    & 74.26          \\ \cdashline{1-5}
+ Instruction Implication   & 3     & 59.49          & 91.46          & 74.10          \\
+ Zero-Shot CoT Implication & 3     & \textbf{59.48} & 91.30          & 73.98          \\
+ Fewshot Implication       & 3     & 60.10          & 92.10          & 73.49          \\ \hline
Pythia (6.9B)               & -     & 65.42          & 94.00          & 65.01          \\
+ Instruction               & 1     & 66.18          & 95.12          & 64.35          \\ 
+ Role                      & 1     & {\ul 63.48}    & \textbf{95.47} & {\ul 69.73}    \\ \cdashline{1-5}
+ Instruction Refine        & 2     & 60.27          & {\ul 93.73}    & 74.47          \\
+ Role Refine               & 2     & {\ul 59.50}    & 93.55          & {\ul 75.78}    \\ \cdashline{1-5}
+ Triple Instruction Refine & 3     & 59.40          & {\ul 93.03}    & 75.53          \\
+ Triple Role Refine        & 3     & 57.87          & 92.89          & \textbf{78.27} \\ \cdashline{1-5}
+ Instruction Implication   & 3     & 58.08          & 90.46          & 75.85          \\
+ Zero-Shot CoT Implication & 3     & \textbf{57.78} & 90.33          & 76.28          \\
+ Fewshot Implication       & 3     & 58.15          & 91.20          & 76.33          \\ \bottomrule
\end{tabular}
}
\end{table}
