# Supplementary material for: Thinking Fair and Slow: On the Efficacy of Structured Prompts for Debiasing Language Models
Source: arXiv:2405.10431 source file (2024-05-16)
Supplement: Supplementary file 3 [file toxicity_table_appendix.tex]

% Please add the following required packages to your document preamble:
% \usepackage{booktabs}
% \usepackage[normalem]{ulem}
% \useunder{\uline}{\ul}{}
\begin{table}[]
\resizebox{0.4\textwidth}{!}{
\begin{tabular}{llll}
\hline
Method                      & Steps & Mean           & Change            \\ \hline
Tiny Llama (1.1B)           & -     & 0.038          & 0.00\%            \\
+ Instruction               & 1     & {\ul 0.042}    & {\ul 11.88\%}     \\
+ Role                      & 1     & 0.042          & 12.11\%           \\ \cdashline{1-4}
+ Instruction Refine        & 2     & {\ul 0.043}    & {\ul 12.28\%}     \\
+ Role Refine               & 2     & 0.043          & 14.65\%           \\ \cdashline{1-4}
+ Triple Instruction Refine & 3     & 0.043          & 12.29\%           \\
+ Triple Role Refine        & 3     & 0.043          & 14.74\%           \\ \cdashline{1-4}
+ Instruction Implication   & 3     & 0.038          & -0.84\%           \\
+ Zero-Shot CoT Implication & 3     & \textbf{0.037} & \textbf{-2.31\%}  \\
+ Fewshot Implication       & 3     & 0.037          & -1.27\%           \\ \hline
GPT2 XL (1.5B)              & -     & 0.051          & 0.00\%            \\
+ Instruction               & 1     & \textbf{0.049} & \textbf{-5.45\%}  \\
+ Role                      & 1     & 0.069          & 34.97\%           \\ \cdashline{1-4}
+ Instruction Refine        & 2     & {\ul 0.057}    & {\ul 11.24\%}     \\
+ Role Refine               & 2     & 0.062          & 20.25\%           \\ \cdashline{1-4}
+ Triple Instruction Refine & 3     & {\ul 0.053}    & {\ul 3.20\%}      \\
+ Triple Role Refine        & 3     & 0.054          & 5.37\%            \\ \cdashline{1-4}
+ Instruction Implication   & 3     & 0.054          & 5.84\%            \\
+ Zero-Shot CoT Implication & 3     & 0.055          & 7.20\%            \\
+ Fewshot Implication       & 3     & 0.053          & 3.54\%            \\ \hline
Pythia (6.9B)               & -     & 0.048          & 0.00\%            \\
+ Instruction               & 1     & \textbf{0.042} & \textbf{-12.81\%} \\ 
+ Role                      & 1     & 0.045          & -6.53\%           \\ \cdashline{1-4}
+ Instruction Refine        & 2     & {\ul 0.043}    & {\ul -12.11\%}    \\
+ Role Refine               & 2     & 0.045          & -6.52\%           \\ \cdashline{1-4}
+ Triple Instruction Refine & 3     & {\ul 0.042}    & {\ul -12.51\%}    \\ 
+ Triple Role Refine        & 3     & 0.045          & -6.53\%           \\ \cdashline{1-4}
+ Instruction Implication   & 3     & 0.046          & -5.10\%           \\
+ Zero-Shot CoT Implication & 3     & 0.045          & -6.20\%           \\
+ Fewshot Implication       & 3     & 0.043          & -11.54\%          \\ \hline
\end{tabular}
}
\end{table}
